# Supplementary material for: Pressure-Driven Phase Evolution and Optoelectronic Properties of Lead-free Halide Perovskite Rb$_2$TeBr$_6$
Source: arXiv:2511.02311 source file (2026-04-17)
Supplement: Supplementary file 1 [file Supplementary__Pressure_Driven_Phase_Evolution_and_Optoelectronic_Properties_of_Lead_free_Halide_Perovskite_Rb_2TeBr_6.pdf]

# Supplementary: Pressure-Driven Phase Evolution and Optoelectronic Properties of Lead-free Halide Perovskite

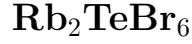

Suvashree Mukherjee,<sup>1,2</sup> Asish Kumar Mishra,<sup>1,2</sup> K.A.

Irshad,<sup>3</sup> Bobby Joseph,<sup>3</sup> and Goutam Dev Mukherjee<sup>1,2,\*</sup>

<sup>1</sup>*Department of Physical Sciences, Indian Institute of Science  
Education and Research Kolkata, Mohanpur Campus,  
Mohanpur 741246, Nadia, West Bengal, India.*

<sup>2</sup>*National Centre for High Pressure Studies,  
Indian Institute of Science Education and Research Kolkata,  
Mohanpur Campus, Mohanpur 741246, Nadia, West Bengal, India.*

<sup>3</sup>*Elettra-Sincrotrone Trieste S.C.p.A.,  
S.S. 14 Km 163.5 in Area Science Park, Basovizza 34149, Italy*

(Dated: November 4, 2025)

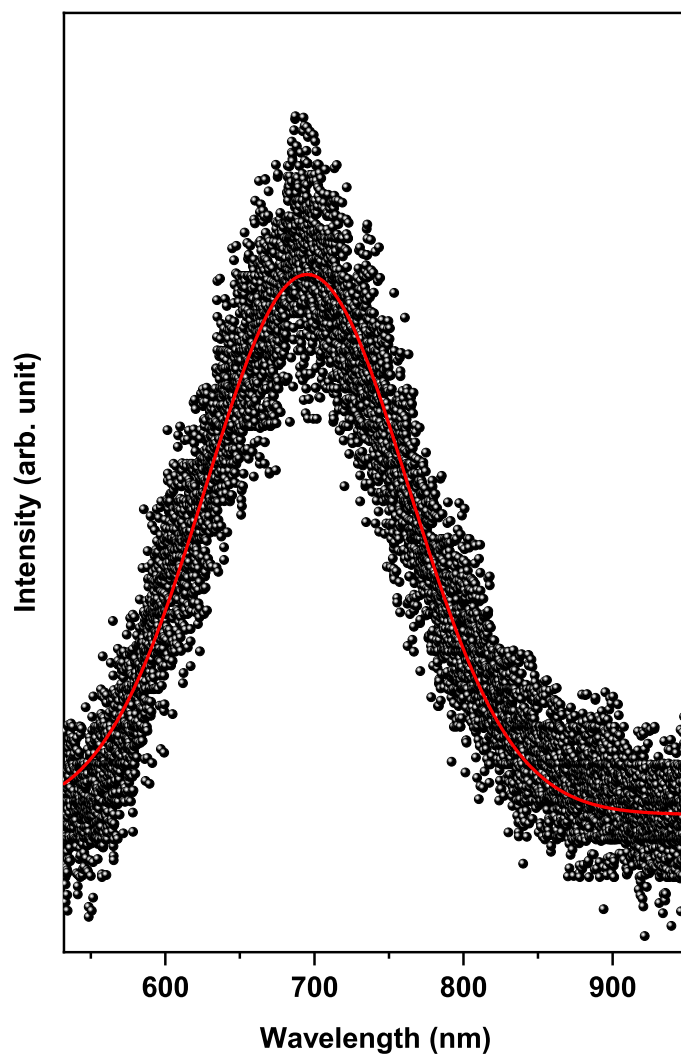

Figure S1: Ambient PL spectrum of  $\text{Rb}_2\text{TeBr}_6$ . The black balls represent the experimental data and the red line shows a fit of the experimental data points to Gaussian function.

---

\* Corresponding author: goutamdev@iiserkol.ac.in

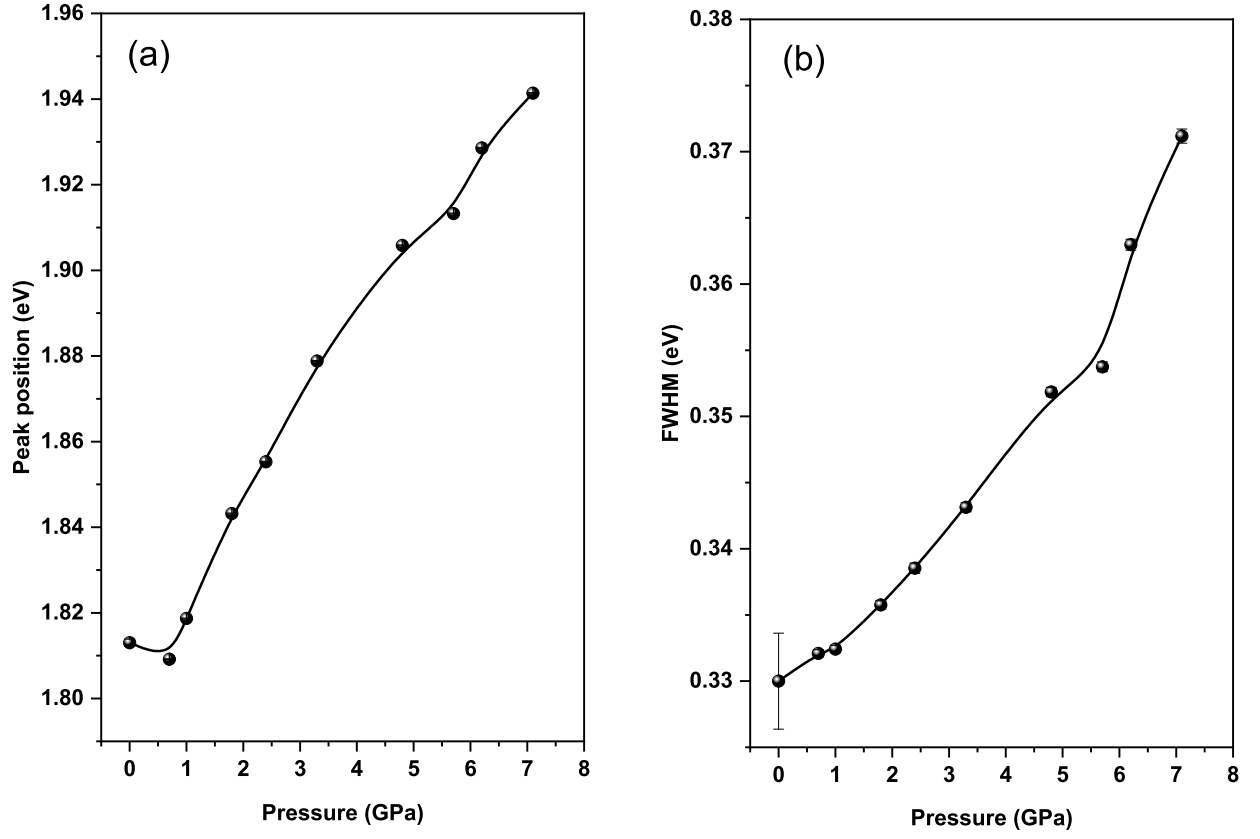

Figure S2(a): Variation of PL peak position (in eV) of  $\text{Rb}_2\text{TeBr}_6$  under pressure, which exhibits a continuous blue shift. (b) The FWHM of PL spectra of  $\text{Rb}_2\text{TeBr}_6$  at different pressure.

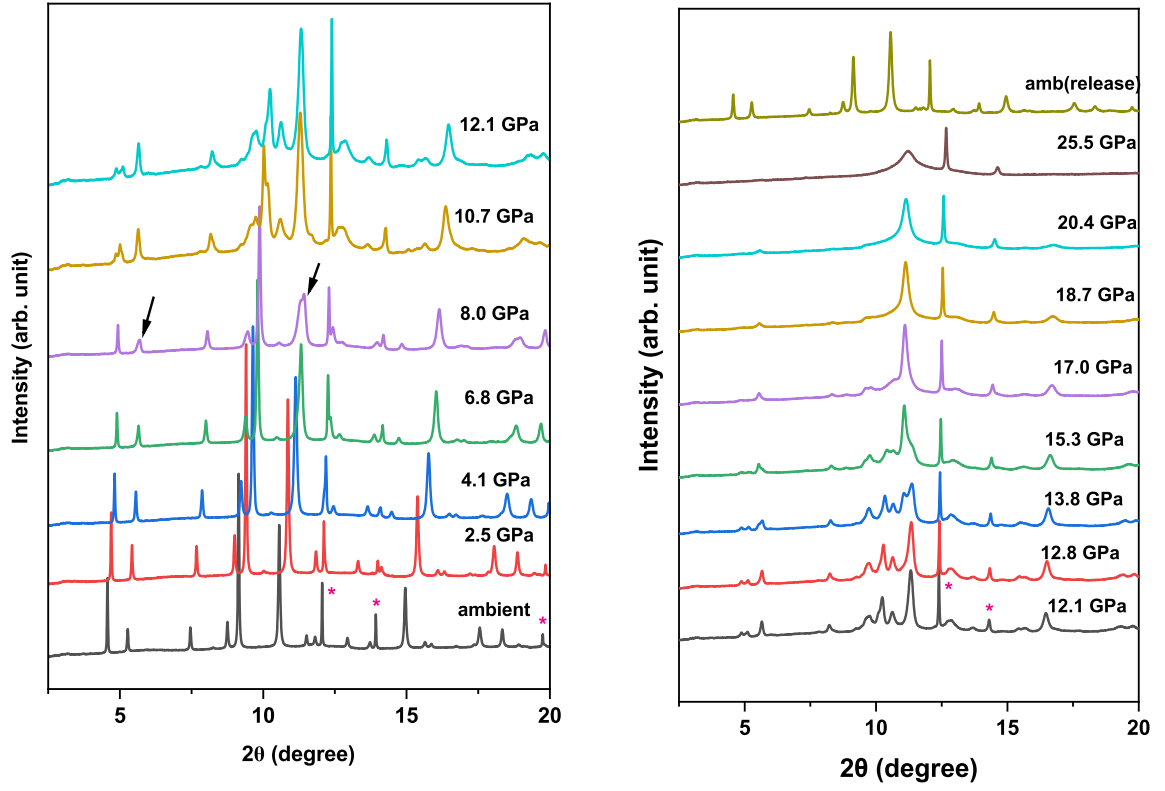

Figure S3: XRD spectra of  $\text{Rb}_2\text{TeBr}_6$  at some selected pressure points. Silver peaks are indicated using stars of magenta colour. The peak broadening at 8.0 GPa are indicated by arrows.

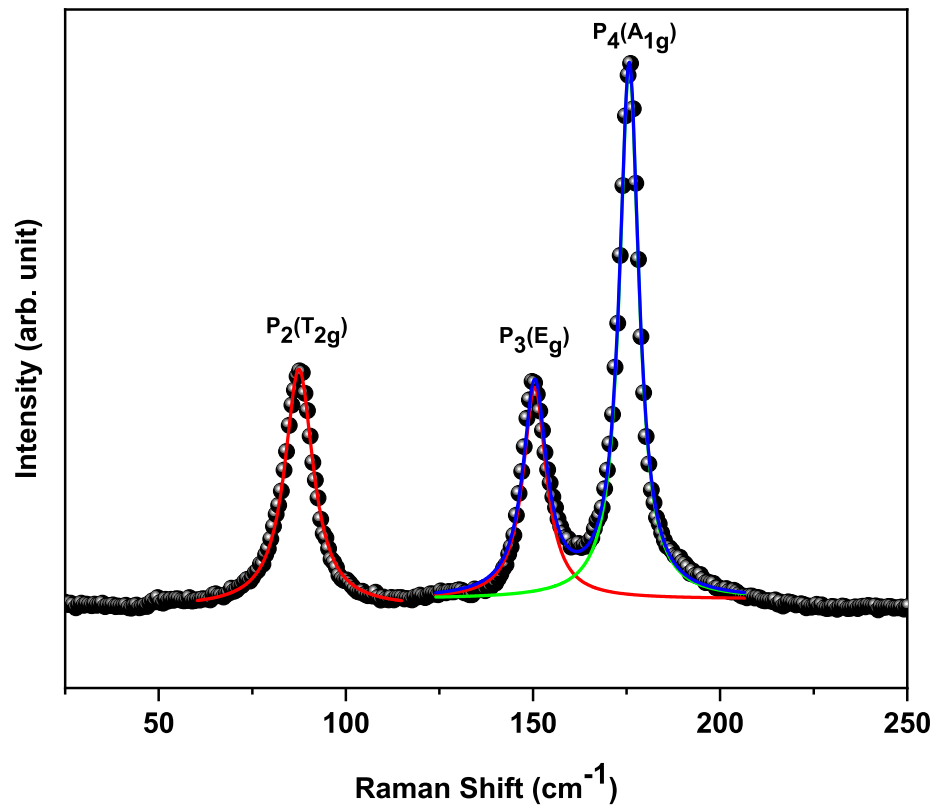

Figure S4: Raman spectrum of  $\text{Rb}_2\text{TeBr}_6$  in ambient condition. The black circles represent the experimental data and the red and blue lines show a fit of experimental data points to Lorentzian functions.

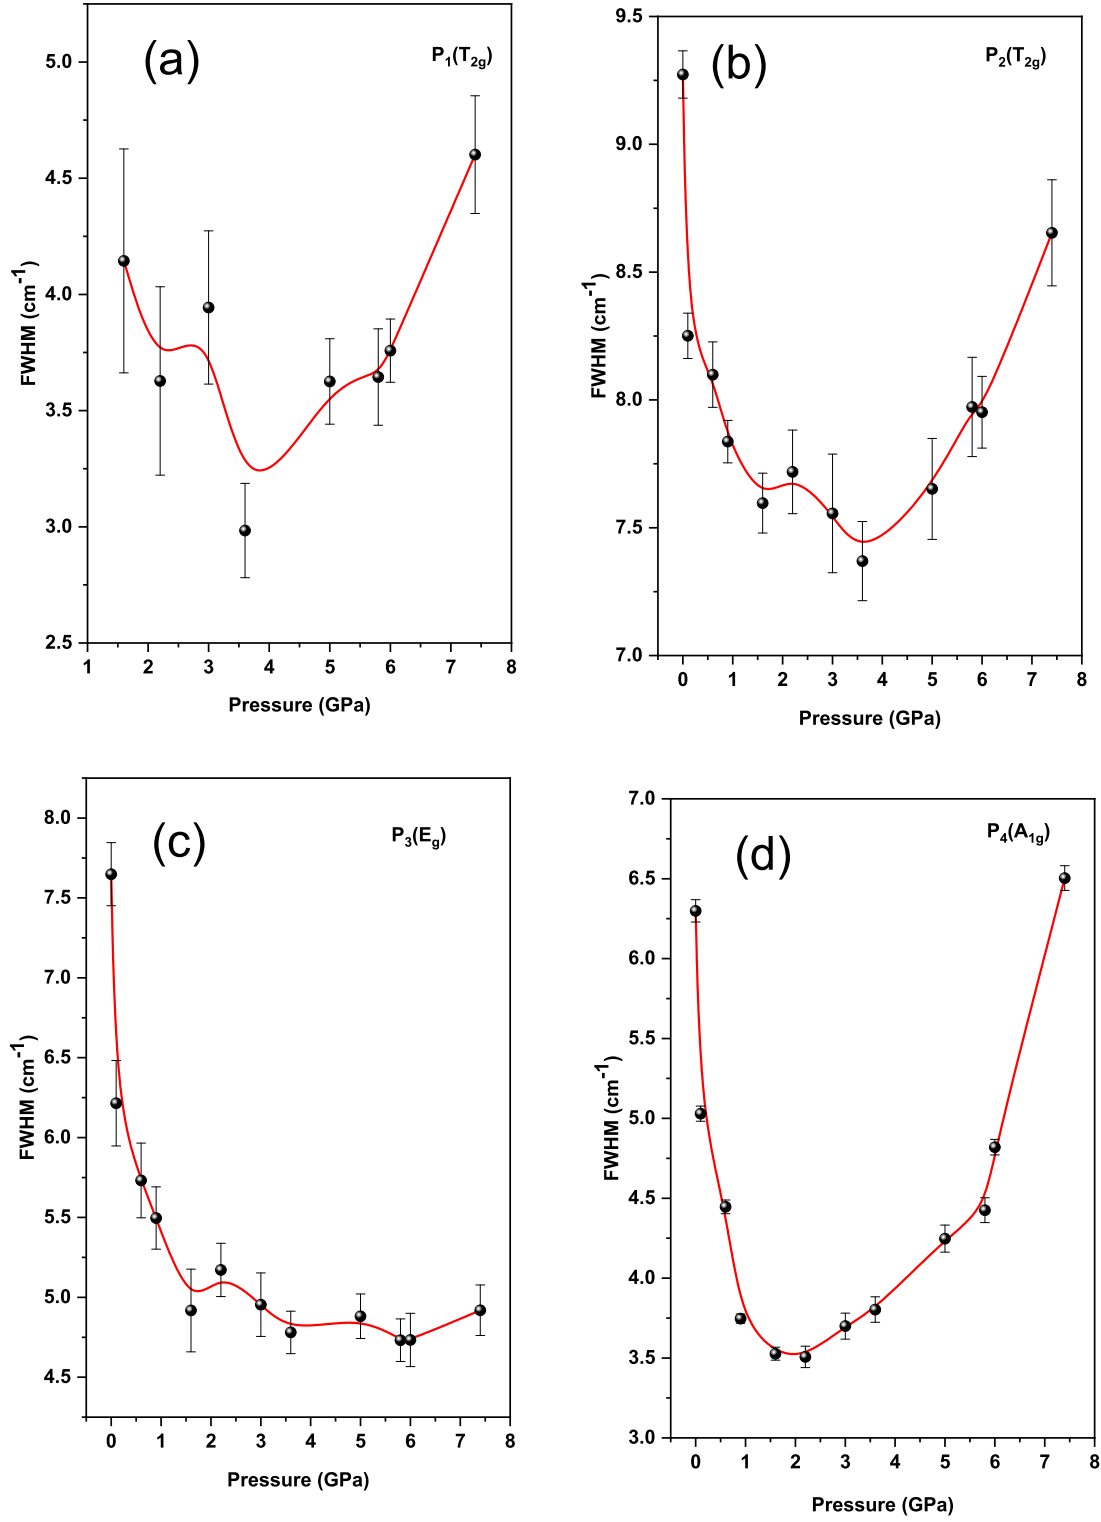

Figure S5: Pressure dependence of the FWHM of Raman modes of Rb<sub>2</sub>TeBr<sub>6</sub> in the cubic phase.

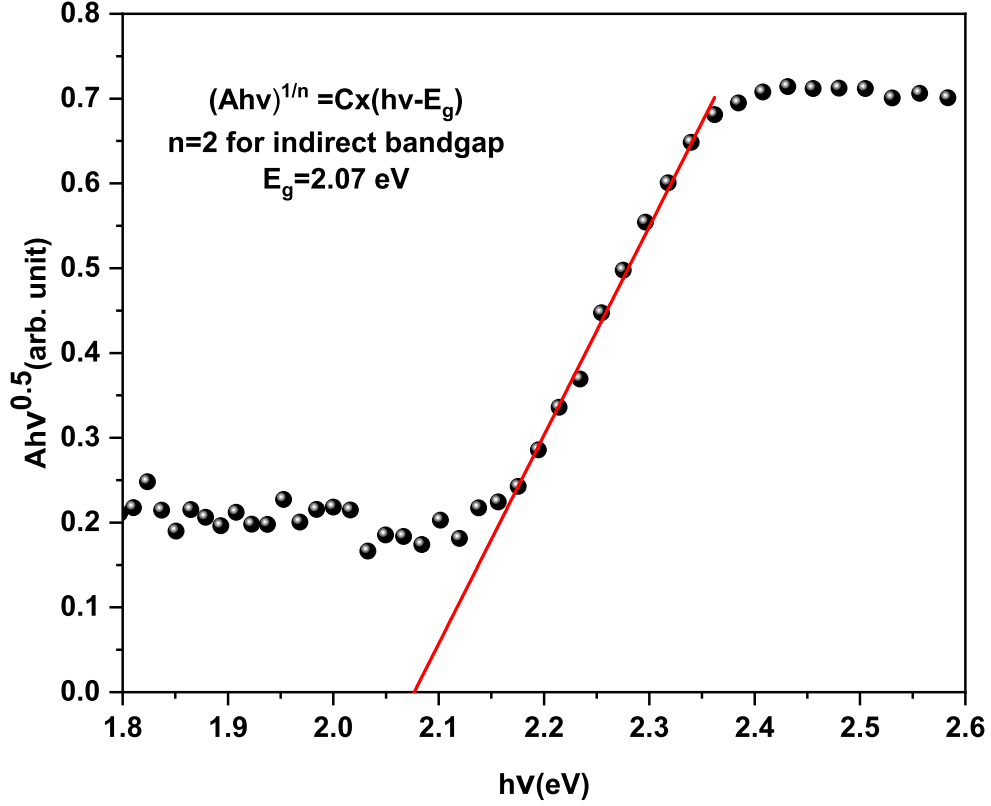

Figure S6: Determination of the optical bandgap of  $\text{Rb}_2\text{TeBr}_6$  from the absorption spectrum in ambient condition.

### STOKES SHIFT AND HUANG–RHYS PARAMETER(S) OF $\text{Rb}_2\text{TeBr}_6$ UNDER PRESSURE

The Stokes shift ( $\Delta E_{\text{Stokes}}$ ) for  $\text{Rb}_2\text{TeBr}_6$  is determined from the optical absorption and photoluminescence (PL) spectra. At ambient pressure,  $\text{Rb}_2\text{TeBr}_6$  exhibits a Stokes shift of 0.60 eV, which decreases monotonically with increasing pressure. The Stokes shift reduces to 0.53 eV at 2.2 GPa, corresponding to the pressure at which the PL intensity reaches its maximum. The Huang–Rhys parameter ( $S$ ) value of  $\text{Rb}_2\text{TeBr}_6$  is evaluated from the Stokes shift using the relation  $\Delta E_{\text{Stokes}} = 2S\hbar\omega_{LO}$ , where  $\hbar$  is the reduced Planck constant and  $\omega_{LO}$  is the longitudinal optical phonon vibration frequency corresponds to the  $A_{1g}$  phonon mode, which dominates the electron–phonon scattering process in halide perovskite [1]. At ambient

pressure, the  $S$  value is 13.8, indicating strong electron–phonon coupling. With compression,  $S$  decreases gradually and reaches 10.9 at 2.2 GPa, coinciding with the pressure at which the maximum PL efficiency is observed. In a similar system,  $\text{Cs}_2\text{TeCl}_6$ , the optimal value for the  $S$  factor is reported to be 12.0 [1].

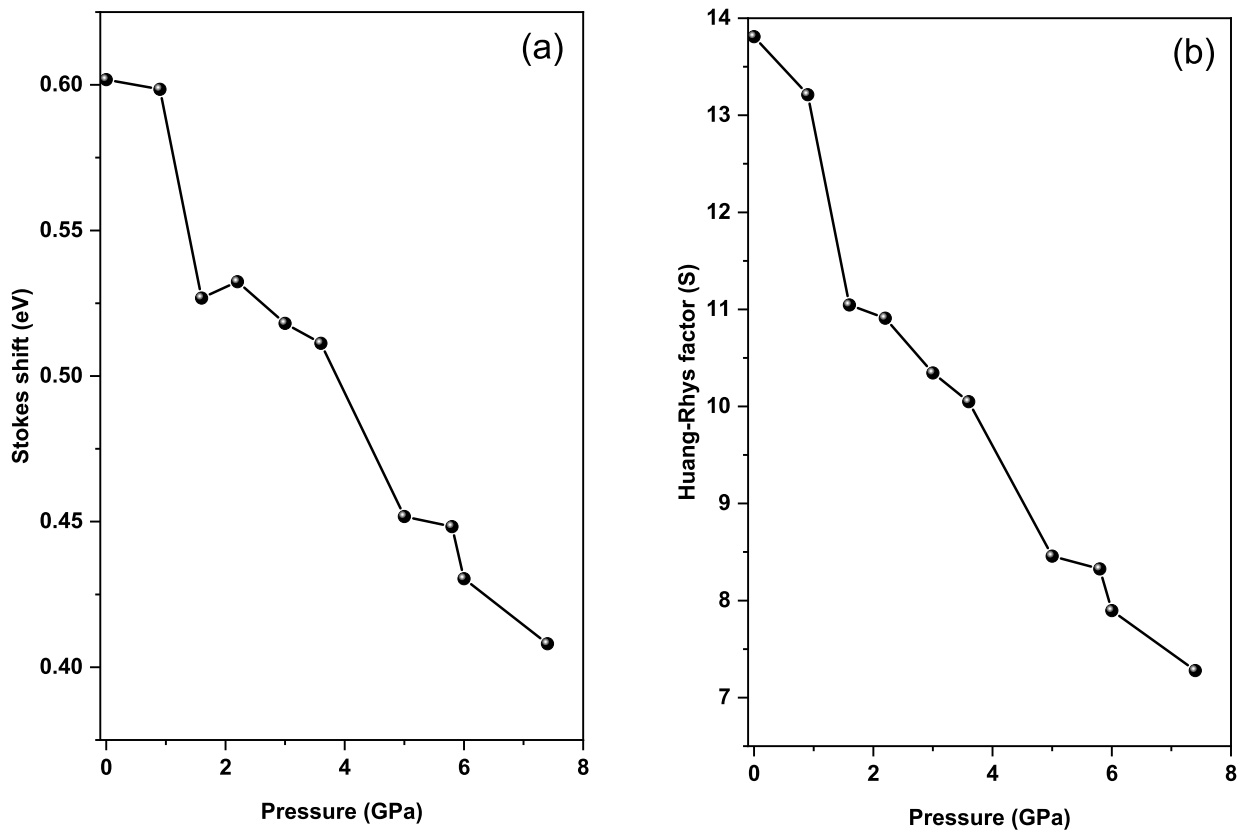

Figure S7(a) Variation of Stokes shift and (b)  $S$  factor with pressure in the cubic phase of  $\text{Rb}_2\text{TeBr}_6$ .

- 
- [1] H. Shi, L. Chen, H. Moutaabbid, Z. Feng, G. Zhang, L. Wang, Y. Li, H. Guo, and C. Liu. *Small*. **20**, 2405692 (2024)
